# Supplementary material for: What's Behind PPO's Collapse in Long-CoT? Value Optimization Holds the Secret
Source: arXiv:2503.01491 source file (2025-03-03)
Supplement: Supplementary file 1 [file appendix.tex]

\section{Hello World}
%\subsection{Hello World}
